# Supplementary material for: Visual Feedback for Players of Multi-Level Capture the Flag Games: Field Usability Study
Source: arXiv:1912.10781 source file (2020-08-27)
Supplement: Supplementary file 1 [file questionaire.pdf]

*The purpose of this research is to study how people interact with the visual user interface of cybersecurity education platform and to collect related data. The benefits I may expect from the study are: (a) an appreciation of the research community, (b) an opportunity to contribute to scientific research, and (c) an opportunity to learn about novel interactive visualizations in cybersecurity visualizations.*

*I also understand that:*

- *By participating in this study, I give consent to processing the data I create*
- *I agree with the mouse movement recording which is embedded in the application;*
- *The anonymized results of this study may be submitted for publication;*
- *The researchers do not foresee any risks to me for participating in this study, nor do they expect that I will experience any discomfort or stress.*
- *I may withdraw from the study at any time;*
- *All of the data collected will remain strictly confidential.*
- *Only people associated with the study will see my responses.*
- *My responses will not be associated with my name; instead, my name will be converted to a code number when the researchers store the data.*
- *Upon completion, I can ask any questions regarding the research topics and my participation upon completion.*

*Involved researchers: <names>*

*Open the Clustering and Timeline views. Spend some time by exploring the visualizations. The Clustering visualization is focused on the reached score while the Timeline visualization detail results from the time perspective and also enables you to explore the results of other players.*

*When ready continue to solving tasks*

*Continue >>>*

# Questionnaire

## T1: Find out when you finished the game.

answer: ________________________________

| | 1 | 2 | 3 | 4 | 5 | 6 |
|---|---|---|---|---|---|---|
| How difficult (1) or easy (6) was to perform this task using selected visualization(s)? | ☐ | ☐ | ☐ | ☐ | ☐ | ☐ |
| How meaningless (1) or meaningful (6) was this task from the game participant's perspective? | ☐ | ☐ | ☐ | ☐ | ☐ | ☐ |
| Which visualization was more helpful to solve the task: | | | | | | |
| Clustering results view (1 = very *useless, I did not use it*, 6 = *very useful*) | ☐ | ☐ | ☐ | ☐ | ☐ | ☐ |
| Timeline results view (1 = very *useless, I did not use it*, 6 = *very useful*) | ☐ | ☐ | ☐ | ☐ | ☐ | ☐ |

Free comments on the clustering results view.
comment: ________________________________

Free comments on the timeline results view.
comment: ________________________________

## T2: Find out in which level(s) you reached the lowest score.

answer: ________________________________

| | 1 | 2 | 3 | 4 | 5 | 6 |
|---|---|---|---|---|---|---|
| How difficult (1) or easy (6) was to perform this task using selected visualization(s)? | ☐ | ☐ | ☐ | ☐ | ☐ | ☐ |
| How meaningless (1) or meaningful (6) was this task from the game participant's perspective? | ☐ | ☐ | ☐ | ☐ | ☐ | ☐ |
| Which visualization was more helpful to solve the task: | | | | | | |
| Clustering results view (1 = very *useless, I did not use it*, 6 = *very useful*) | ☐ | ☐ | ☐ | ☐ | ☐ | ☐ |
| Timeline results view (1 = very *useless, I did not use it*, 6 = *very useful*) | ☐ | ☐ | ☐ | ☐ | ☐ | ☐ |

Free comments on the clustering results view.
comment: ________________________________

Free comments on the timeline results view.
comment: ________________________________

## T3: Find out your final score.

answer: ________________________________

| | 1 | 2 | 3 | 4 | 5 | 6 |
|---|---|---|---|---|---|---|
| How difficult (1) or easy (6) was to perform this task using selected visualization(s)? | ☐ | ☐ | ☐ | ☐ | ☐ | ☐ |
| How meaningless (1) or meaningful (6) was this task from the game participant's perspective? | ☐ | ☐ | ☐ | ☐ | ☐ | ☐ |
| Which visualization was more helpful to solve the task: | | | | | | |
| Clustering results view (1 = very *useless, I did not use it*, 6 = *very useful*) | ☐ | ☐ | ☐ | ☐ | ☐ | ☐ |
| Timeline results view (1 = very *useless, I did not use it*, 6 = *very useful*) | ☐ | ☐ | ☐ | ☐ | ☐ | ☐ |

Free comments on the clustering results view.
comment: ________________________________

Free comments on the timeline results view.
comment: ________________________________

## T4: Find out how much time you spent in the 2nd level.

answer: ________________________________

| | 1 | 2 | 3 | 4 | 5 | 6 |
|---|---|---|---|---|---|---|
| How difficult (1) or easy (6) was to perform this task using selected visualization(s)? | ☐ | ☐ | ☐ | ☐ | ☐ | ☐ |
| How meaningless (1) or meaningful (6) was this task from the game participant's perspective? | ☐ | ☐ | ☐ | ☐ | ☐ | ☐ |
| Which visualization was more helpful to solve the task: | | | | | | |
| Clustering results view (1 = very *useless, I did not use it*, 6 = *very useful*) | ☐ | ☐ | ☐ | ☐ | ☐ | ☐ |
| Timeline results view (1 = very *useless, I did not use it*, 6 = *very useful*) | ☐ | ☐ | ☐ | ☐ | ☐ | ☐ |

Free comments on the clustering results view.
comment: ________________________________

Free comments on the timeline results view.
comment: ________________________________

## T5: Find out when you advanced from 2nd to 3rd level.

answer: ________________________________

| | 1 | 2 | 3 | 4 | 5 | 6 |
|---|---|---|---|---|---|---|
| How difficult (1) or easy (6) was to perform this task using selected visualization(s)? | ☐ | ☐ | ☐ | ☐ | ☐ | ☐ |
| How meaningless (1) or meaningful (6) was this task from the game participant's perspective? | ☐ | ☐ | ☐ | ☐ | ☐ | ☐ |
| Which visualization was more helpful to solve the task: | | | | | | |
| Clustering results view (1 = very *useless, I did not use it*, 6 = *very useful*) | ☐ | ☐ | ☐ | ☐ | ☐ | ☐ |
| Timeline results view (1 = very *useless, I did not use it*, 6 = *very useful*) | ☐ | ☐ | ☐ | ☐ | ☐ | ☐ |

Free comments on the clustering results view.
comment: ________________________________

Free comments on the timeline results view.
comment: ________________________________

## T6: Find out in which level you lost most points in the game.

answer: ________________________________

| | 1 | 2 | 3 | 4 | 5 | 6 |
|---|---|---|---|---|---|---|
| How difficult (1) or easy (6) was to perform this task using selected visualization(s)? | ☐ | ☐ | ☐ | ☐ | ☐ | ☐ |
| How meaningless (1) or meaningful (6) was this task from the game participant's perspective? | ☐ | ☐ | ☐ | ☐ | ☐ | ☐ |
| Which visualization was more helpful to solve the task: | | | | | | |
| Clustering results view (1 = very *useless, I did not use it*, 6 = *very useful*) | ☐ | ☐ | ☐ | ☐ | ☐ | ☐ |
| Timeline results view (1 = very *useless, I did not use it*, 6 = *very useful*) | ☐ | ☐ | ☐ | ☐ | ☐ | ☐ |

Free comments on the clustering results view.
comment: ________________________________

Free comments on the timeline results view.
comment: ________________________________

## T7: Characterize your score compared to other players.

- ☐ I reached higher score than most players
- ☐ I reached a rather high score
- ☐ My score was rather average
- ☐ I reached a rather lower score
- ☐ I reached lower score than most players

| | **1** | **2** | **3** | **4** | **5** | **6** |
|---|---|---|---|---|---|---|
| How difficult (1) or easy (6) was to perform this task using selected visualization(s)? | ☐ | ☐ | ☐ | ☐ | ☐ | ☐ |
| How meaningless (1) or meaningful (6) was this task from the game participant's perspective? | ☐ | ☐ | ☐ | ☐ | ☐ | ☐ |
| Which visualization was more helpful to solve the task: | | | | | | |
| Clustering results view (1 = very *useless, I did not use it*, 6 = *very useful*) | ☐ | ☐ | ☐ | ☐ | ☐ | ☐ |
| Timeline results view (1 = very *useless, I did not use it*, 6 = *very useful*) | ☐ | ☐ | ☐ | ☐ | ☐ | ☐ |

Free comments on the clustering results view.
comment: ________________________________

Free comments on the timeline results view.
comment: ________________________________

## T8: Characterize your time spent by playing compared to other players.

- ☐ I was one of the fastest players
- ☐ I was quite fast
- ☐ My time was rather average
- ☐ I was quite slow
- ☐ I was one of the slowest players

| | **1** | **2** | **3** | **4** | **5** | **6** |
|---|---|---|---|---|---|---|
| How difficult (1) or easy (6) was to perform this task using selected visualization(s)? | ☐ | ☐ | ☐ | ☐ | ☐ | ☐ |
| How meaningless (1) or meaningful (6) was this task from the game participant's perspective? | ☐ | ☐ | ☐ | ☐ | ☐ | ☐ |
| Which visualization was more helpful to solve the task: | | | | | | |
| Clustering results view (1 = very *useless, I did not use it*, 6 = *very useful*) | ☐ | ☐ | ☐ | ☐ | ☐ | ☐ |
| Timeline results view (1 = very *useless, I did not use it*, 6 = *very useful*) | ☐ | ☐ | ☐ | ☐ | ☐ | ☐ |

Free comments on the clustering results view.
comment: ________________________________

Free comments on the timeline results view.
comment: ________________________________

## T9: Find out the player who reached the closest score to your score.

answer: ________________________________

| | 1 | 2 | 3 | 4 | 5 | 6 |
|---|---|---|---|---|---|---|
| How difficult (1) or easy (6) was to perform this task using selected visualization(s)? | ☐ | ☐ | ☐ | ☐ | ☐ | ☐ |
| How meaningless (1) or meaningful (6) was this task from the game participant's perspective? | ☐ | ☐ | ☐ | ☐ | ☐ | ☐ |
| Which visualization was more helpful to solve the task: | | | | | | |
| Clustering results view (1 = very *useless, I did not use it*, 6 = *very useful*) | ☐ | ☐ | ☐ | ☐ | ☐ | ☐ |
| Timeline results view (1 = very *useless, I did not use it*, 6 = *very useful*) | ☐ | ☐ | ☐ | ☐ | ☐ | ☐ |

Free comments on the clustering results view.
comment: ________________________________

Free comments on the timeline results view.
comment: ________________________________

## T10: Find out how much time was assigned for playing the game.

answer: ________________________________

| | 1 | 2 | 3 | 4 | 5 | 6 |
|---|---|---|---|---|---|---|
| How difficult (1) or easy (6) was to perform this task using selected visualization(s)? | ☐ | ☐ | ☐ | ☐ | ☐ | ☐ |
| How meaningless (1) or meaningful (6) was this task from the game participant's perspective? | ☐ | ☐ | ☐ | ☐ | ☐ | ☐ |
| Which visualization was more helpful to solve the task: | | | | | | |
| Clustering results view (1 = very *useless, I did not use it*, 6 = *very useful*) | ☐ | ☐ | ☐ | ☐ | ☐ | ☐ |
| Timeline results view (1 = very *useless, I did not use it*, 6 = *very useful*) | ☐ | ☐ | ☐ | ☐ | ☐ | ☐ |

Free comments on the clustering results view.
comment: ________________________________

Free comments on the timeline results view.
comment: ________________________________

## T11: Is there somebody who reached a high score in a significantly short time? If so insert his Player ID.

answer: ________________________________

| | 1 | 2 | 3 | 4 | 5 | 6 |
|---|---|---|---|---|---|---|
| How difficult (1) or easy (6) was to perform this task using selected visualization(s)? | ☐ | ☐ | ☐ | ☐ | ☐ | ☐ |
| How meaningless (1) or meaningful (6) was this task from the game participant's perspective? | ☐ | ☐ | ☐ | ☐ | ☐ | ☐ |
| Which visualization was more helpful to solve the task: | | | | | | |
| Clustering results view (1 = very *useless, I did not use it*, 6 = *very useful*) | ☐ | ☐ | ☐ | ☐ | ☐ | ☐ |
| Timeline results view (1 = very *useless, I did not use it*, 6 = *very useful*) | ☐ | ☐ | ☐ | ☐ | ☐ | ☐ |

Free comments on the clustering results view.
comment: ________________________________

Free comments on the timeline results view.
comment: ________________________________

## T12: Find out who reached the best score.

answer: ________________________________

| | 1 | 2 | 3 | 4 | 5 | 6 |
|---|---|---|---|---|---|---|
| How difficult (1) or easy (6) was to perform this task using selected visualization(s)? | ☐ | ☐ | ☐ | ☐ | ☐ | ☐ |
| How meaningless (1) or meaningful (6) was this task from the game participant's perspective? | ☐ | ☐ | ☐ | ☐ | ☐ | ☐ |
| Which visualization was more helpful to solve the task: | | | | | | |
| Clustering results view (1 = very *useless, I did not use it*, 6 = *very useful*) | ☐ | ☐ | ☐ | ☐ | ☐ | ☐ |
| Timeline results view (1 = very *useless, I did not use it*, 6 = *very useful*) | ☐ | ☐ | ☐ | ☐ | ☐ | ☐ |

Free comments on the clustering results view.
comment: ________________________________

Free comments on the timeline results view.
comment: ________________________________

# Demographic questions

## Age

## Gender

- ☐ Female
- ☐ Male
- ☐ Prefer not to say

## Highest educational qualification

- ☐ Elementary school
- ☐ High school / Secondary school
- ☐ University graduate (bachelor or master degree)
- ☐ Postgraduate qualification

## Exposure to the technology

| | **Don’t own one** | **Daily use** | **Weekly use** | **Rarely use** |
|---|---|---|---|---|
| Smartphone | ☐ | ☐ | ☐ | ☐ |
| Laptop | ☐ | ☐ | ☐ | ☐ |
| Desktop | ☐ | ☐ | ☐ | ☐ |
| Tablet | ☐ | ☐ | ☐ | ☐ |

## Familiarity with cybersecurity topics

- ☐ Newcomer
- ☐ Novice user
- ☐ Experienced user
- ☐ Security professional
